# Supplementary material for: Measurement of three-dimensional inclusive muon-neutrino charged-current cross sections on argon with the MicroBooNE detector
Source: arXiv:2307.06413 ancillary file (2025-11-26)
Supplement: Supplementary file 1 [file Supplemental.pdf]

# Supplemental Materials: Measurement of three-dimensional inclusive muon-neutrino charged-current cross sections on argon with the MicroBooNE detector

August 30, 2024

## I. SMOOTHING OF DETECTOR SYSTEMATIC UNCERTAINTIES

This section provides a detailed description of how the Gaussian Processes Regression (GPR) smoothing algorithm [1–3] is used to reduce the overestimation of detector systematic uncertainties that result from a limited quantity of Monte Carlo (MC) simulation available. A bootstrapping procedure, discussed extensively in Ref. [4] and briefly reviewed here, is used to estimate the uncertainty in the detector response.

This process involves comparing the distribution of events simulated using nominal detector response parameter values to the distribution of events simulated using detector response parameter values under offsets constructed by observing the difference between data and nominal MC prediction [5]. The dataset used in this comparison consists of cosmic rays that cross either the anode or cathode plane to enable accurate reconstruction. These offsets are treated as $1\sigma$ variations, and each pair of distributions, under nominal and offset detector response parameter values, is referred to as one "universe". The difference between the nominal and $1\sigma$ distributions is referred to as $\vec{V}_D$, and the average difference over all universes is referred to as $\vec{V}_D^{\text{nominal}}$. A covariance matrix $M_R$ is computed from the set of all difference vectors $\vec{V}_D$ to represent the uncertainty in estimating $\vec{V}_D^{\text{nominal}}$. Since there is a limited quantity of simulation available, there are statistical fluctuations present in the set of $\vec{V}_D$, and therefore in the computation of $M_R$. This problem is amplified in multiple dimensions, where the large number of bins further restricts the number of events per bin. The smoothing procedure aims to address the large statistical fluctuations present by describing the set of $\vec{V}_D$ and corresponding $M_R$ with a smooth distribution.

In general, GPR aims to produce a smoothed prediction over a target set of points, $\vec{x}_a$, by incorporating information from measurements, $\vec{y}_b$, at positions $\vec{x}_b$. Note that the subscripts $a$ and $b$ are used to identify the distribution being referenced, while $i$ and $j$, shown later, are used to identify a particular bin within a distribution. GPR begins with an uninformed prior of a joint normal distribution with a zero mean vector and an identity covariance matrix, $p(\vec{x}) = N_{\vec{x}}(\vec{0}, I)$, on the target distribution as well as the measured distribution. The measurement $\vec{y}_b$ and corresponding covariance $\Sigma_y$ are used in combination with a kernel matrix $\Sigma_K$ to generate an updated posterior prediction $p(\vec{x}_a|\vec{x}_b)$ with mean $\vec{\mu}_{a|b}$ and covariance $\Sigma_{T,a|b}$. The kernel matrix describes the level of correlation between any two bins, and is computed using a kernel function $K(\vec{x}_i, \vec{x}_j)$. By choosing a function that decays with distance, the physical intuition of smoothness can be applied by treating nearby bins as highly correlated. The kernel matrix is added to the measured covariance to form a total covariance $\Sigma_T$:

$$\Sigma_{K;ij} = K(\vec{x}_i, \vec{x}_j), \tag{1}$$

$$\Sigma_T = \Sigma_y + \Sigma_K. \tag{2}$$

From these, Bayes' theorem is used to compute the posterior distribution:

$$p(\vec{x}_a|\vec{x}_b) = N_{x_a}(\vec{\mu}_{a|b}, \Sigma_{T,a|b}) \tag{3}$$

where the mean and covariance are computed using:

$$\vec{\mu}_{a|b} = \vec{\mu}_a + \Sigma_{K,ab}\Sigma_{T,bb}^{-1}(\vec{y}_b - \vec{\mu}_b), \tag{4}$$

$$\Sigma_{T,a|b} = \Sigma_{K,aa} - \Sigma_{K,ab}\Sigma_{T,bb}^{-1}\Sigma_{K,ba}. \tag{5}$$

Here $\vec{\mu}_a$ and $\vec{\mu}_b$ are the prior means at points $\vec{x}_a$ and $\vec{x}_b$, respectively.

From Eq. (4), we can see that the difference between measured and predicted values, $\vec{y}_b - \vec{\mu}_b$, is used to update the mean prediction. However, measurements with large uncertainty will contribute less to the posterior distribution, as the term $\Sigma_{T,bb}^{-1}$ will be suppressed. This mathematical framework used to compute the posterior distribution is identical to that in Sec. II in the conditional constraint formalism. This work computes the posterior prediction over the target distribution at the same bin centers as used in the measured distribution $\vec{y}_b = \vec{V}_D^{\text{nominal}}$, i.e $\vec{x}_a = \vec{x}_b$.

However, in principle the GPR technique can be used to obtain predictions using any set of points, not just at $\vec{x}_b$. The kernel function is computed using a radial basis function (RBF), which asserts the intuition of smoothness by assigning a correlation that decays exponentially as the distance squared between bin centers increases:

$$K(\vec{x}_i, \vec{x}_j) = e^{-|(\vec{x}_i - \vec{x}_j)\cdot\vec{s}|^2/2}, \tag{6}$$

$$s_k = \frac{1}{L_k}. \tag{7}$$

The bin centers $\vec{x}_i$ and $\vec{x}_j$ are three-dimensional vectors describing their location within the kinematic phase space. Here, $L_k$ denotes a characteristic length scale for each dimension over which the points are sufficiently correlated. The RBF kernel considers very close points to be highly correlated, and is strictly decreasing as a function of distance between points as it exponentially decays towards zero, treating distant points as almost fully uncorrelated. This causes nearby points to play a significant role in shaping the posterior prediction at a given location, while distant points have almost no effect, as can be seen in Eq. (4), where $\Sigma_K$ acts on the measurement $(\vec{y}_b - \vec{\mu}_b)$.

In the reported work, the RBF kernel utilizes three characteristic length scales for the neutrino energy, muon momentum, and muon forward angle axes. Based on the measured kinematic resolutions, length scales were chosen to be 0.1 in $\cos(\theta_\mu^{\rm rec})$ and relative 20% for each of $E_\nu^{\rm rec}$ and $P_\mu^{\rm rec}$, the latter achieved by using a length scale of $\ln(1.2)$ and natural log values of $E_\nu^{\rm rec}$ and $P_\mu^{\rm rec}$ in $\vec{x}_i$ and $\vec{x}_j$ in Eq. (6). Given the length scales and measured data, Eq. (4) and Eq. (5) therefore directly give us the mean and covariance of the smoothed posterior prediction. These become the new values for $\vec{V}_D^{\rm nominal}$ and $M_R$, and consequently reduce the detector uncertainty by a factor of twenty from ≈400% to ≈20%, reducing the overestimation of uncertainties from finite MC simulation statistics. The detector response uncertainties computed with the use of smoothing in this three-dimensional measurement were compared to counterparts on single-differential measurements [6], where statistical fluctuations are small and smoothing was not used. In all cases, the detector response uncertainties in this three-dimensional analysis were found to be comparable or larger than those counterparts, demonstrating that smoothing has not suppressed the uncertainty estimation beyond what is achieved in a high statistics scenario. The impact of smoothing can be seen in Fig. 1, which also shows the breakdown of uncertainties from each source over the 138 analysis bins in true space. To help understand the overall magnitude of uncertainties across the truth phase space, Fig. 2 presents the total fractional uncertainty in each analysis bin. Even after using GPR smoothing, detector response uncertainties are still the second largest source of uncertainties in the analysis behind statistical uncertainties.

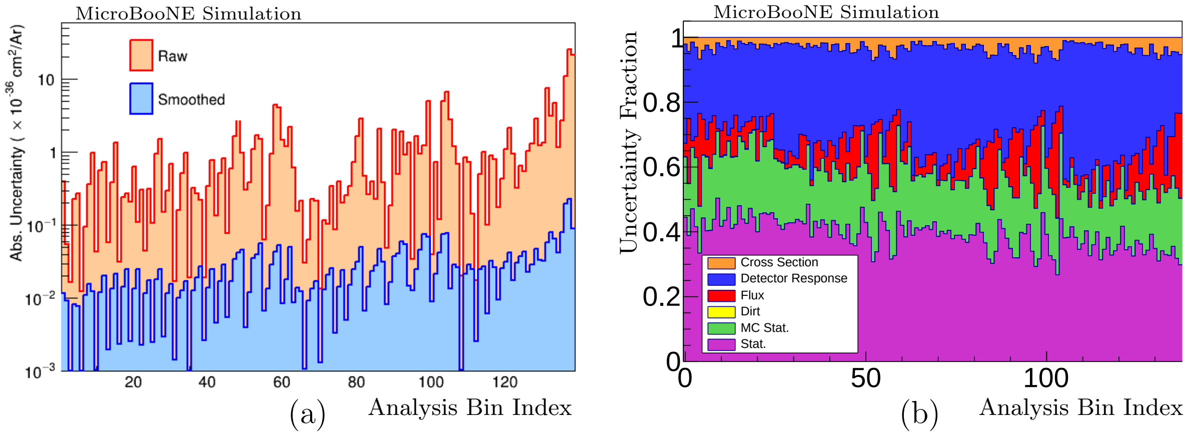


FIG. 1. a) Comparison of the detector response diagonal uncertainties in the cases with and without the use of GPR smoothing, demonstrating an order of magnitude reduction in detector response uncertainty estimation. b) Breakdown of total uncertainties across the various statistical and systematic sources, including the use of GPR smoothing in the estimation of the detector response uncertainty, plotted as a fraction of the total diagonal uncertainty in each bin.

## II. VALIDATION OF OVERALL MODEL

To ensure that the unfolded cross sections are not biased beyond the estimated uncertainties, it is important to demonstrate that the MicroBooNE model prediction and uncertainties cover the distribution seen in data. This

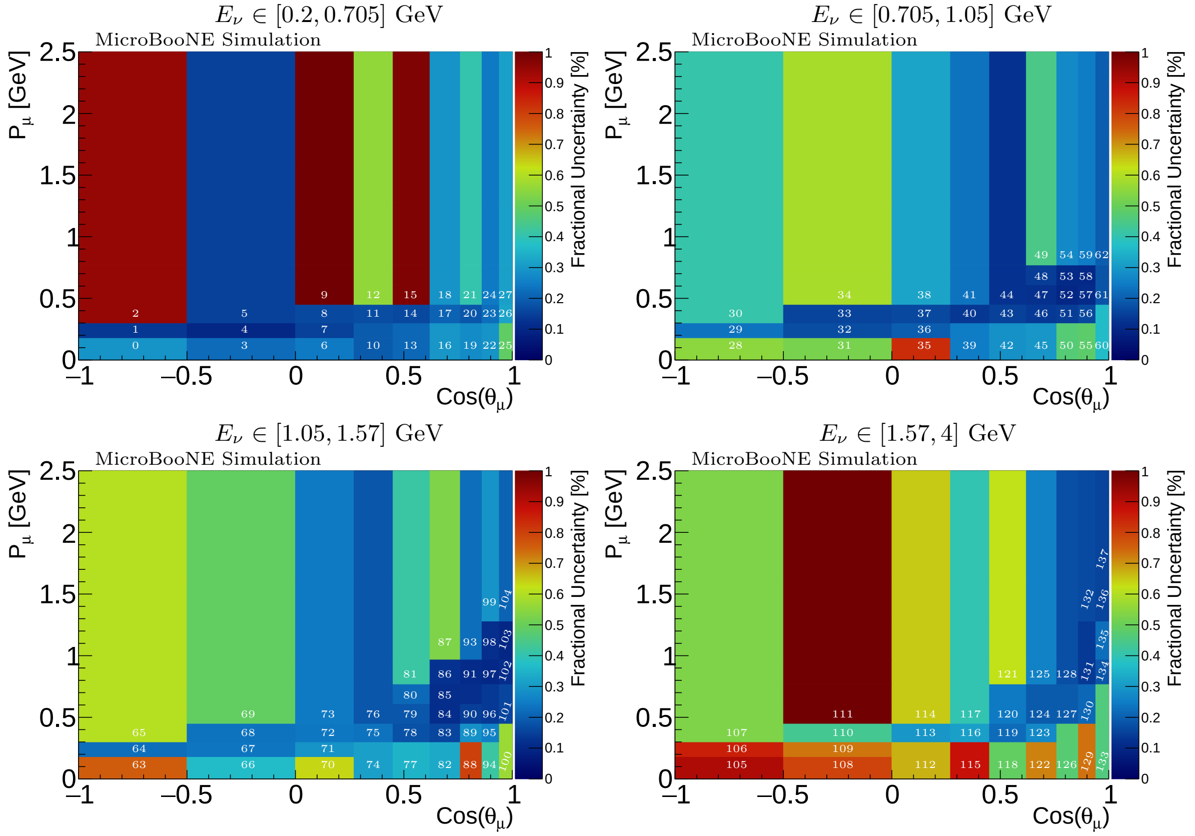


FIG. 2. Total uncertainty as a fraction of the predicted cross section from the MicroBooNE model in the corresponding bin. The four sub-figures each present a different $E_\nu$ slice. The total uncertainty comes from the square root of the covariance matrix diagonal entries. Analysis bin number overlaid on top of each bin near the bottom.

ensures that the MicroBooNE model is a reliable estimate of the response matrix used in unfolding. We use a validation procedure to evaluate the signal and background model prediction $(P)$'s capability to describe the data measurement $(M)$ within $P$'s uncertainty through a $\chi^2$ goodness-of-fit (GoF) test, based on the test statistic:

$$\chi^2 = (M-P)^T \times C_{\rm full}^{-1}(M,P) \times (M-P), \tag{8}$$

where the covariance matrix $C_{\rm full}^{-1}$ is the full covariance matrix including both statistical and systematic uncertainties. To validate the model across the full three-dimensional phase space $\{E_\nu, P_\mu, \cos(\theta_\mu)\}$, it is important to maintain a nonzero efficiency. The selection efficiency across the phase space is shown in Fig. 3. For a given bin in truth variables, the selection efficiency is computed as the ratio of selected to total events with truth kinematics corresponding to that bin.

The GoF test evaluates the null hypothesis that the overall model prediction, including uncertainties, is able to cover the distribution seen in data. Note that here by model we refer to the central value along with its uncertainties. This evaluation can be narrowed to a specific portion of modeling by using the conditional covariance matrix formalism [7], which uses Bayes' theorem similar to how it is used in Sec. I. Let $\mu$ and $\Sigma$ represent the central value and covariance predicted by the model over two channels U and V, with corresponding data measurement $n$:

$$\Sigma = \begin{pmatrix} \Sigma^{UU} & \Sigma^{UV} \\ \Sigma^{VU} & \Sigma^{VV} \end{pmatrix}. \tag{9}$$

For example, the $U$ channel could represent the distribution of events over $E_{\rm had}^{\rm rec}$, while the $V$ channel could represent the distribution of events over $P_\mu^{\rm rec}$. Then we can derive the posterior prediction on $U$ given the constraints on $V$:

$$\begin{aligned} \mu^{U,\rm constrained} &= \mu^U + \Sigma^{UV} \times \left(\Sigma^{VV}\right)^{-1} \times \left(n^V - \mu^V\right), \\ \Sigma^{UU,\rm constrained} &= \Sigma^{UU} - \Sigma^{UV} \times \left(\Sigma^{VV}\right)^{-1} \times \Sigma^{VU}. \end{aligned} \tag{10}$$

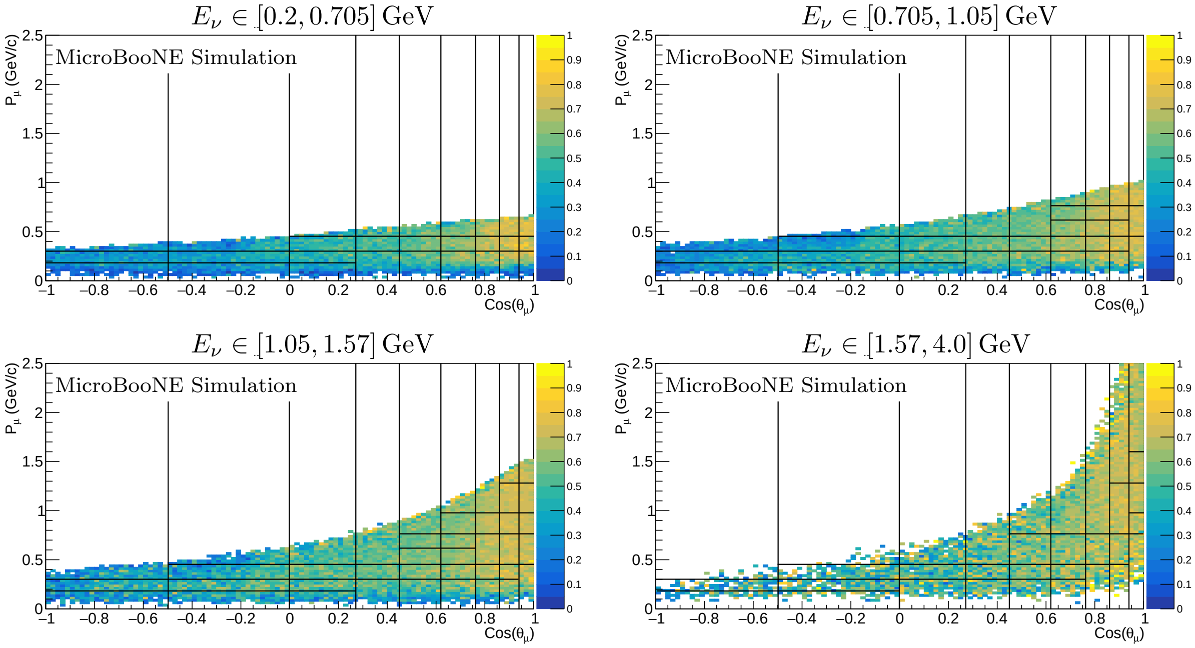


FIG. 3. Selection efficiency for simulated events over $\{P_\mu,\, \cos(\theta_\mu)\}$ within each $E_\nu$ slice. Bin edges are indicated by black lines. Bins containing under 5 events in truth are not drawn because of their low statistics.

Following the example distributions chosen above, the muon momentum measurement would be used as a constraint on the hadronic energy prediction, updating the model prediction on hadronic energy to exclude regions in disagreement with the measurement over muon momentum. A GoF test can be performed on $V$ first, and then performed on $U$ while using the data distribution on $V$ as a constraint. This allows for examination of the modeling of the correlated predictions over $U$ and $V$.

In particular, this allows us to evaluate the GoF of the distribution over $\{E^{\mathrm{rec}}_{\mathrm{had}}, \cos(\theta^{\mathrm{rec}}_\mu)\}$ using $\{P^{\mathrm{rec}}_\mu, \cos(\theta^{\mathrm{rec}}_\mu)\}$ as a constraint. Note that since the inclusive $\nu_\mu$ CC channel is described by three degrees of freedom, it is not possible to form independent three-dimensional channels $U$ and $V$, and so no three-dimensional constrained GoF test can be performed. Therefore, the two-dimensional channels used provide the best test of the kinematic phase space. There are key features of the conditional constraint procedure and corresponding validation tests over distributions of hadronic energy that are worth mentioning in detail. First, the posterior model prediction on $U$ given the constraint on $V$ will have greatly reduced uncertainties. This is because the model predictions and their uncertainties over various kinematic distributions are correlated, so that restricting the allowed phase space of model parameters to fit the data on $V$ also constrains the model prediction on $U$. As a result, the common systematic uncertainties between $U$ and $V$ are greatly reduced for the posterior prediction on $V$.

This results in a validation test that is more sensitive to mismodeling than the overall unfolded measurement, which uses the default MicroBooNE model without application of the conditional constraint procedure during the unfolding. For example, large correlated neutrino flux uncertainties can hide issues in the modeling of missing hadronic energy. A basic GoF test may not detect this mismodeling, but the unfolded measurement may still be affected. However, through the conditional covariance formalism, correlated neutrino flux uncertainties between the muon kinematics and hadronic energy are removed, allowing the mismodeling to be detected by the constrained GoF test. This fact is demonstrated through fake data studies in section III, where model validation tests on fake data are able to detect significant mismodeling before the bias introduced is larger than the uncertainties on the unfolded measurement.

In the case of the model validation of the hadronic energy prediction, the use of the muon kinematics measurement as a constraint allows for validation of the correlations between the muon kinematics and hadronic energy modeling. This is particularly important because it creates a GoF test on the constrained model prediction over the $\{E^{\mathrm{rec}}_{\mathrm{had}}, \cos(\theta^{\mathrm{rec}}_\mu)\}$ distribution that is sensitive to the modeling of missing energy, allowing for the mapping from energy transfer $\nu$ to $E^{\mathrm{rec}}_{\mathrm{had}}$ to be validated. This point can be seen intuitively in two ways.

First, through conservation of energy the sensitivity to the modeling of $E^{\mathrm{missing}}_{\mathrm{had}}$ can be seen:

$$E_\nu = E_\mu + E^{\mathrm{rec}}_{\mathrm{had}} + E^{\mathrm{missing}}_{\mathrm{had}}. \tag{11}$$

$E^{\mathrm{rec}}_{\mathrm{had}}$ is directly measured, $E_\mu$ is determined through the measurement of $P^{\mathrm{rec}}_\mu$, and the distribution over $E_\nu$ is

controlled by the flux prediction, which is constrained by the muon kinematics measurements. This leaves $E_{\rm had}^{\rm missing}$ as the only undetermined quantity, meaning that the constrained GoF test is sensitive to its mismodeling.

Second, the model predictions over $E_{\rm had}^{\rm missing}$, $E_{\rm had}^{\rm rec}$, and $P_\mu^{\rm rec}$ are correlated as a result of simulating the underlying neutrino interaction channels such as quasi-elastic (QE), resonance (RES), and deep inelastic scattering (DIS). Additionally, the $\{P_\mu^{\rm rec}, \cos(\theta_\mu^{\rm rec})\}$ measurement constrains the space of model variations across the interaction channels, creating an effect similar to re-weighting the hadronic system using the muon kinematics as a sideband. Furthermore, the model predictions over interaction channels each vary as a function of the muon scattering angle $\theta_\mu^{\rm rec}$, forming detailed sets of predictions in two dimensions. This allows the constrained GoF test in two dimensions to perform a detailed examination of the model performance, going beyond the level of validation possible in one dimension. As a result, the constrained GoF test over $\{E_{\rm had}^{\rm rec}, \cos(\theta_\mu^{\rm rec})\}$ tests the modeling of correlations between the kinematic distributions, making it sensitive to the modeling of $E_{\rm had}^{\rm missing}$.

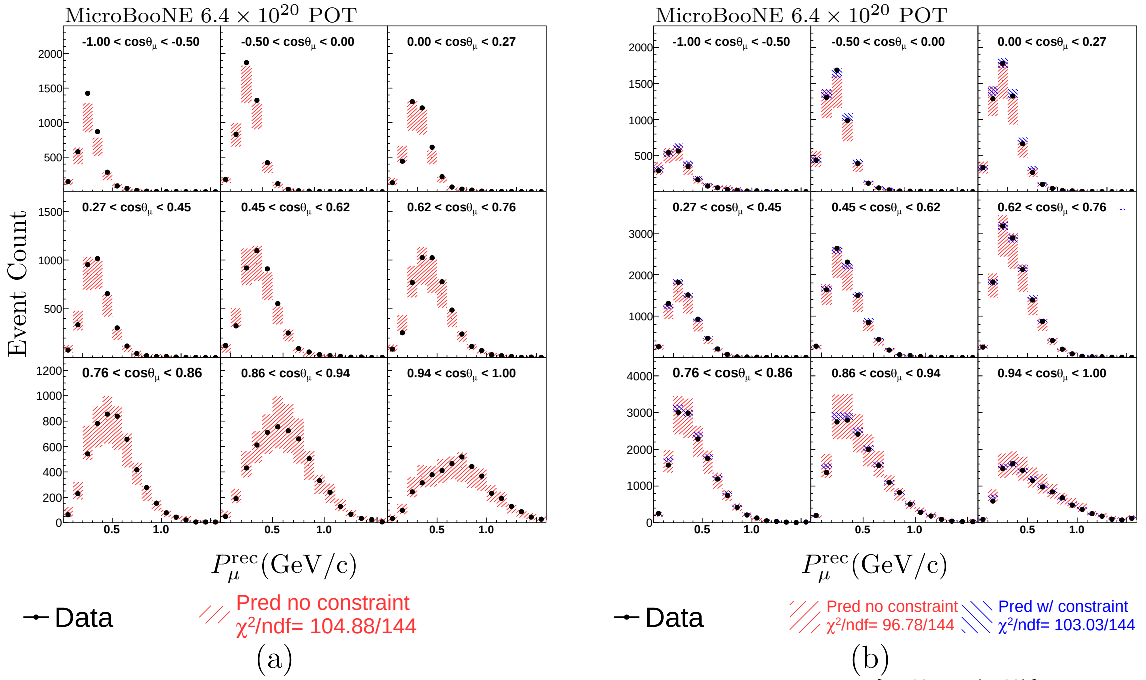


FIG. 4. Comparison between data and prediction over the muon kinematic distribution $\{P_\mu^{\rm rec}, \cos(\theta_\mu^{\rm rec})\}$ for fully contained events in (a) and partially contained events in (b). The fully contained distribution is used as a constraint on the model prediction for the partially constrained distribution following Eq. 10. The statistical and systematic uncertainties of the data and simulation are included in the uncertainty bands shown with the model prediction.

Figure 4 demonstrates model validation over the muon kinematic distribution $\{P_\mu^{\rm rec}, \cos(\theta_\mu^{\rm rec})\}$, and Fig. 5 demonstrates model validation over $\{E_{\rm had}^{\rm rec}, \cos(\theta_\mu^{\rm rec})\}$. In all cases, the model validation tests find that the model prediction contains enough uncertainties to describe the distribution seen in data, with $\chi^2$/ndf values less than 1. If any corresponding p-values are outside $2\sigma$, the `MicroBooNE model` is determined to fail model validation, requiring the model to be sufficienctly expanded before proceeding with unfolding. By contrast, since the `MicroBooNE model` passed all model validation tests, it can confidently be used in unfolding.

## III. FAKE DATA STUDIES

Fake data studies are used to verify the sensitivity of the data-driven model validation. In the previous analysis [8], fake data studies were performed on single-dimensional distributions. In this analysis, additional fake data studies are performed featuring an unfolding to the three-dimensional analysis binning. For each fake data study, we examine whether the `MicroBooNE model` is able to describe the distribution of fully contained events, partially contained events, and the joint distribution of fully contained and partially contained events. For a fake data study to pass validation, the p-value for an associated GoF test must be more extreme than the p-value of the corresponding extracted cross section, demonstrating that we are able to detect the mismodeling at a higher significance than is found in the unfolded measurement. This ensures that if such a mismodeling were present in the data to a degree that would significantly bias the unfolded measurement, we would have previously detected it in the model validation

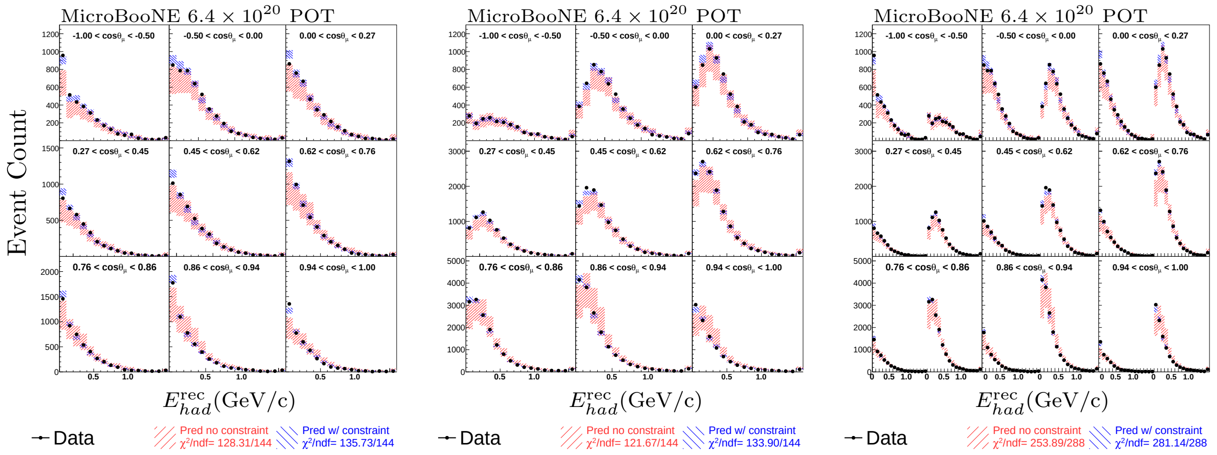


(a) (b) (c)

FIG. 5. Comparison between data and prediction over the 2D distribution $\{E^{\text{rec}}_{\text{had}}, \cos(\theta^{\text{rec}}_{\mu})\}$ for (a) fully contained events, (b) partially contained events, and (c) both, with the fully contained distribution to the left of the partially contained distribution within each subplot. The red (blue) band gives the uncertainty before (after) applying the 2D $\{P^{\text{rec}}_{\mu}, \cos(\theta^{\text{rec}}_{\mu})\}$ distribution as a constraint on the model prediction following Eq. 10. The statistical and systematic uncertainties of the data and simulation are included in the uncertainty bands shown with the model prediction.

tests.

Because these fake data studies only feature differences in cross section modeling (and event generation in the case of NuWro), we compliment the suite of tests performed using all uncertainties, which parallel those in the previous section, with a parallel series of tests that only use cross section and statistical uncertainties. This provides the strictest criteria for a fake data study to pass model validation, as each distribution is evaluated both under the narrow set of uncertainties that pertain to the variations induced, as well as the full set of uncertainties that provide a direct counterpart to the model validation tests on data. Since model validation is only considered to pass if all tests pass, the presentation of distributions is limited to only those demonstrating the largest mismodeling for each fake data study.

The `NuWro 19.02.01` model provides an independent alternative cross section prediction to the one provided by GENIE v3.0.6 in the `MicroBooNE model`. To test this prediction, a `NuWro` dataset corresponding to $6.1 \times 10^{20}$ POT of data is simulated and used in a fake data study. Model validation tests are performed on the joint distribution of partially and fully contained events, shown in Fig. 6, and the distribution of partially contained events, shown in Fig. 7, both including a version containing all uncertainties and a version containing only cross section and statistical uncertainties. The model performance is observed over the $\{E_{\text{had}}, \cos(\theta_{\mu})\}$ distribution before and after applying the fake data $\{P_{\mu}, \cos(\theta_{\mu})\}$ distribution as a constraint.

With only cross section and statistical uncertainties, the constrained model validation test detects the mismodeling with a $\chi^2$/ndf of 375.51/288 and corresponding p-value of 0.0004. If this level of disagreement (above $2\sigma$) were found in real data, the model would have to be expanded before confidently being used in unfolding. An example of this procedure in practice can be found in [9] that investigated in detail the hadronic final state. In the case of this `NuWro` fake data study, unfolding is still performed to investigate the degree of bias introduced, which yields a $\chi^2$/ndf of 147.9/138 and corresponding p-value of 0.267 when compared to the statistically independent `NuWro` model truth prediction. This demonstrates the improved sensitivity of the constrained GoF test, which detects the mismodeling beyond $3\sigma$, while the unfolded measurement remains well under $2\sigma$. Using all model uncertainties, GoF tests do not detect mismodeling and yield a $\chi^2$/ndf of 125.18/144 and corresponding p-value of 0.87, and the bias in the unfolded measurement is within uncertainties with a $\chi^2$/ndf of 95.4/138 and corresponding p-value of 0.998.

One potential source of mismodeling is the distribution of energy transfer into its visible and missing components. To examine the impact of mismodeling in this mapping on the unfolded measurement, a series of fake data studies are performed by varying the reconstructed proton energy on a per-event basis. This is conducted in 5% increments, from 70% scaling, representing an excess of missing energy, to 130% scaling, representing a deficit of missing energy compared to the `MicroBooNE model` prediction. Like with the `NuWro` fake data study, GoF tests and unfolded cross sections are computed both using the full uncertainties in the model and using only cross section and statistical uncertainties.

The mismodeling detected in GoF tests, performed on the partially contained $\{E_{\text{had}}, \cos(\theta_{\mu})\}$ distribution under constraint by the $\{P_{\mu}, \cos(\theta_{\mu})\}$ distribution, as well as the bias in the extracted cross section, can be found in Table I.

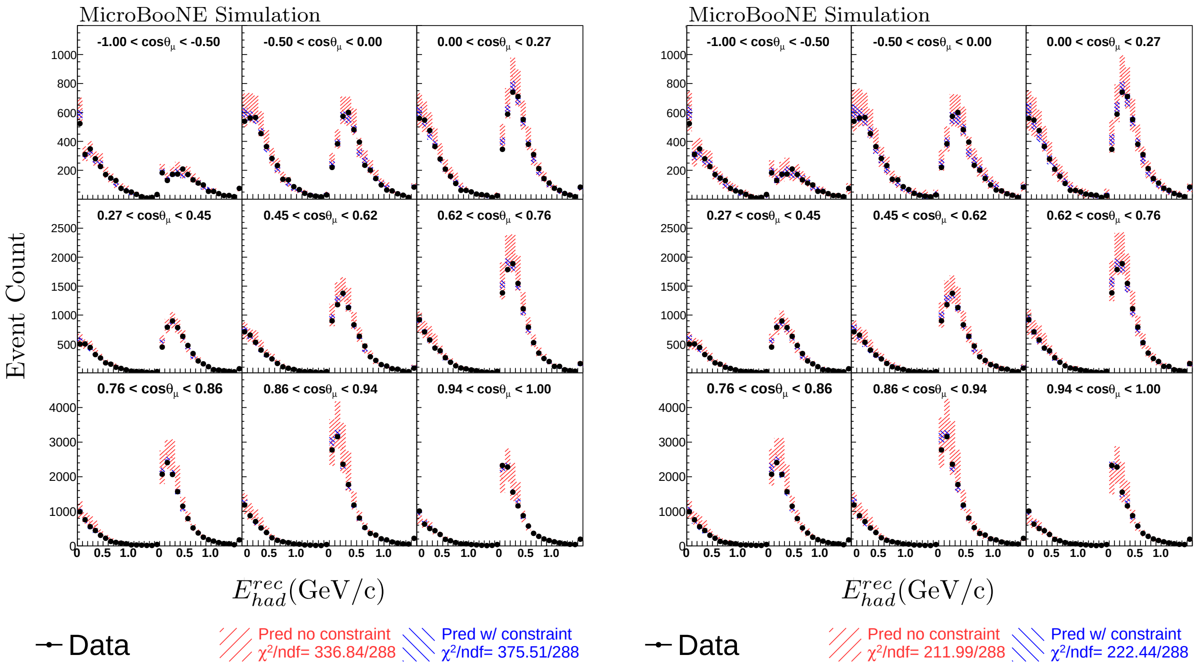


(a) (b)

FIG. 6. Comparison of the joint distribution of partially contained and partially contained events between NuWro fake data and model and prediction using (a) cross section and statistical uncertainties and (b) all uncertainties over the 2D distribution $\{E^{\rm rec}_{\rm had}, \cos(\theta^{\rm rec}_\mu)\}$. Within each angle slice, the fully contained event distribution is shown on the left and the partially contained event distribution is shown on the right. The red (blue) band gives the uncertainty before (after) applying the 2D $\{P^{\rm rec}_\mu, \cos(\theta^{\rm rec}_\mu)\}$ distribution as a constraint on the model prediction following Eq. 10. The statistical and systematic uncertainties of the data and simulation are included in the uncertainty bands shown with the model prediction.

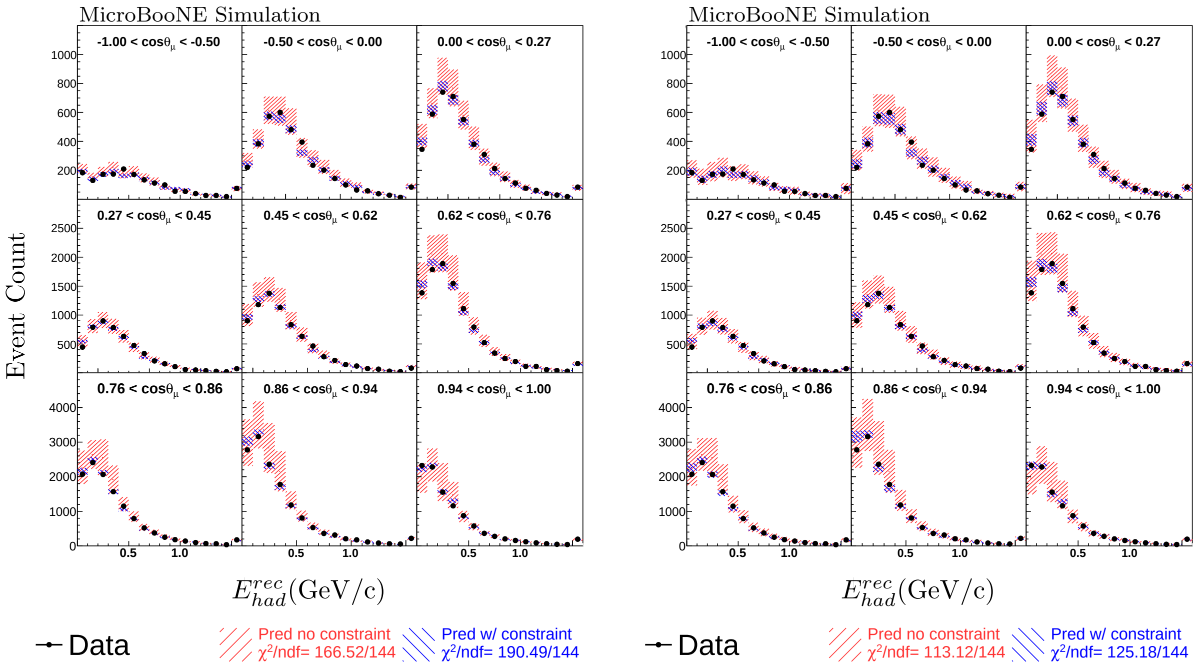


(a) (b)

FIG. 7. Comparison on the distribution of partially contained events between NuWro fake data and model and prediction using (a) cross section and statistical uncertainties and (b) all uncertainties over the 2D distribution $\{E^{\rm rec}_{\rm had}, \cos(\theta^{\rm rec}_\mu)\}$. The red (blue) band gives the uncertainty before (after) applying the 2D $\{P^{\rm rec}_\mu, \cos(\theta^{\rm rec}_\mu)\}$ distribution as a constraint on the model prediction following Eq. 10. The statistical and systematic uncertainties of the data and simulation are included in the uncertainty bands shown with the model prediction.

TABLE I. Model validation goodness-of-fit (GoF) tests compared against bias in extracted cross section measurements using the 138 analysis bins of the 3D measurement. Fake data sets are used, consisting of simulation from the `MicroBooNE model` under various proton energy scalings from 70% to 130%. GoF tests are performed on the partially contained $\{E_{\text{had}}^{\text{rec}}, \cos(\theta_\mu^{\text{rec}})\}$ distribution, using the $\{P_\mu^{\text{rec}}, \cos(\theta_\mu^{\text{rec}})\}$ distribution as a constraint.

| $E_p$ Scaling (%) | Cross Section & Stat Unc. GoF $\chi^2$ (p-value) 144 DoF | Cross Section & Stat Unc. Cross Section Bias $\chi^2$ (p-value) 138 DoF | All Uncertainties GoF $\chi^2$ (p-value) 144 DoF | All Uncertainties Cross Section Bias $\chi^2$ (p-value) 138 DoF |
|---|---|---|---|---|
| 70 | 554.6 ($2 \times 10^{-49}$) | 240.7 ($1.4 \times 10^{-7}$) | 216.4 ($9.5 \times 10^{-5}$) | 126.3 (0.753) |
| 75 | 365.9 ($3 \times 10^{-21}$) | 162.1 (0.08) | 147.7 (0.40) | 85.5 (1) |
| 80 | 225.4 ($1.7 \times 10^{-5}$) | 104.5 (0.985) | 95.8 (0.999) | 55.5 (1) |
| 85 | 123.6 (0.89) | 60.1 (1) | 55.8 (1) | 32.6 (1) |
| 90 | 58.1 (1) | 27.4 (1) | 29.0 (1) | 14.8 (1) |
| 95 | 17.0 (1) | 7.2 (1) | 9.2 (1) | 3.7 (1) |
| 105 | 18.7 (1) | 7.5 (1) | 11.0 (1) | 3.8 (1) |
| 110 | 48.3 (1) | 26.8 (1) | 26.1 (1) | 14.0 (1) |
| 115 | 96.9 (0.999) | 62.3 (1) | 52.6 (1) | 32.3 (1) |
| 120 | 152.7 (0.29) | 104.3 (0.985) | 82.7 (1) | 53.7 (1) |
| 125 | 217.4 ($8 \times 10^{-5}$) | 159.2 (0.105) | 114.3 (0.967) | 81.4 (1) |
| 130 | 289.5 ($9 \times 10^{-12}$) | 229.6 ($1.6 \times 10^{-6}$) | 151.4 (0.321) | 115.6 (0.917) |

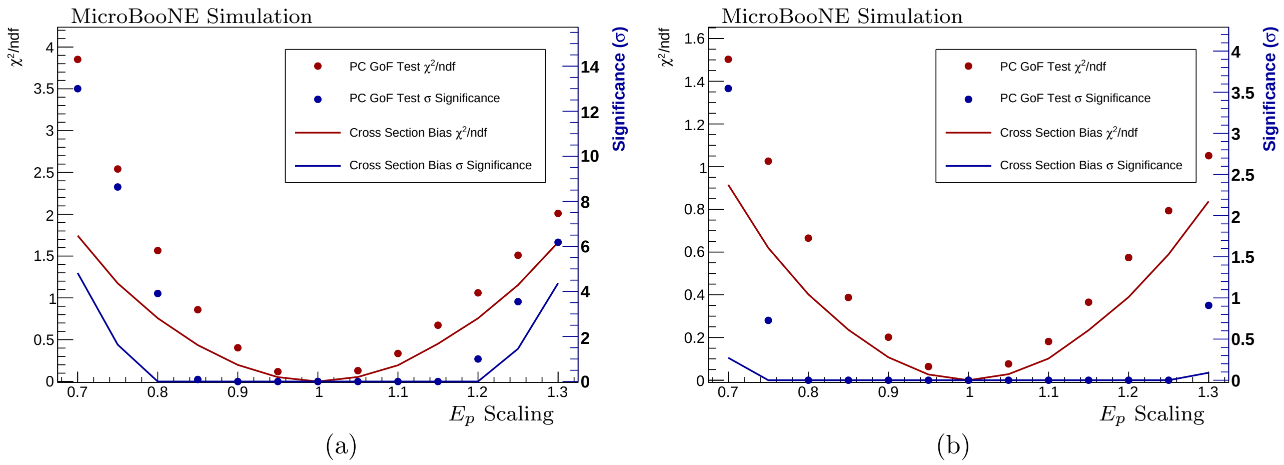


FIG. 8. Comparison between GoF test results and extracted cross section bias for various proton energy scalings, using (a) cross section and statistical uncertainties only, and (b) all uncertainties.

The partially contained distribution is highlighted because it is found to be more sensitive to mismodeling than other distributions in these specific fake data studies. In the case of cross section and statistical uncertainties, the constrained GoF tests detect the mismodeling at -20% proton energy with a $\chi^2$/ndf of 225.4/144 and corresponding p-value of $1.7 \times 10^{-5}$ and at +25% proton energy with a $\chi^2$/ndf of 217.4/144 and corresponding p-value of $8 \times 10^{-5}$. Meanwhile, the respective extracted cross sections both demonstrate lower $\chi^2$/ndf ratios and corresponding p-values within $2\sigma$. When all uncertainties are included, the constrained GoF tests begin to detect mismodeling at -25% and +30%, while the extracted cross section remains within uncertainties with corresponding p-values below $2\sigma$ across the full range of proton energy scalings. Furthermore, Fig. 8 contains the same information as Table I and visually shows that the GoF tests contain larger $\chi^2$/ndf values and statistical significances than the corresponding extracted cross section for all proton energy scalings under both uncertainty treatments.

## IV. FORMATION OF MASTER EQUATION TO UNFOLD THREE-DIMENSIONAL CROSS SECTIONS

In this section we provide the exact mathematical derivation for the cross section unfolding procedure in multiple dimensions. The derivation for the cross section unfolding in the case of one dimension is given in the supplemental material of the previous work [8]. The process of extracting information about the truth content of the measurement bins, given the observed measurements, is referred to as "unfolding." For a typical data unfolding problem, the

formation of the master equation

$$M = R \cdot S \tag{12}$$

is crucial. Here $M$ is the measurable quantity (typically a vector) in the reconstructed kinematics variable space. $S$ is the physics quantity (typically also a vector) to be extracted in the true kinematic variable space, which is the goal of the unfolding procedure. Then the response matrix $R$, which is assumed to be known, connects the unknown $S$ with the actual measurement $M$, and can be determined from theoretical modeling or simulation. As discussed in Sec. II, in this work the estimation of $R$ through the use of the MicroBooNE model is extensively validated. This gives confidence that the unfolding performed based on this estimation of $R$ will not introduce bias beyond the uncertainty shown on the measurement.

In this section, we describe the exact formalism to form the master equation (Eq. 12) for the extraction of the three-dimensional cross section on neutrino energy $E_\nu$ and two kinematic variables $K$ and $P$. $M$ represents the measured number of events as a function of the reconstructed neutrino energy $E_\nu^{\mathrm{rec}}$ and kinematic variables $K^{\mathrm{rec}}$ and $P^{\mathrm{rec}}$:

$$M\left(E_\nu^{\mathrm{rec}}, K^{\mathrm{rec}}, P^{\mathrm{rec}}\right) = N \cdot T \cdot \int\int\int F\left(E_\nu\right) \cdot \frac{d^2\sigma\left(E_\nu, K, P\right)}{dKdP} \cdot D \cdot \epsilon \cdot dE_\nu \cdot dK \cdot dP + B\left(E_\nu^{\mathrm{rec}}, K^{\mathrm{rec}}, P^{\mathrm{rec}}\right), \tag{13}$$

where $N$ and $T$ represent the integrated protons on target (POT) and the number of target nucleons respectively. $F\left(E_\nu\right)$ is the muon neutrino flux as a function of true neutrino energy $E_\nu$. The differential cross section $\frac{d^2\sigma(E_\nu,K,P)}{dKdP}$ is a function of true energy $E_\nu$, $K$ and $P$. The detector response matrix $D$ [or $D\left(E_\nu, E_\nu^{\mathrm{rec}}, K, K^{\mathrm{rec}}, P, P^{\mathrm{rec}}\right)$] is a function of $E_\nu$, $E_\nu^{\mathrm{rec}}$, $K$, $K^{\mathrm{rec}}$, $P$, and $P^{\mathrm{rec}}$, and represents smearing of the neutrino energy reconstruction. The selection efficiency $\epsilon$ [or $\epsilon\left(E_\nu, K, K^{\mathrm{rec}}, P, P^{\mathrm{rec}}\right)$] is a function of $E_\nu$, $K$, $K^{\mathrm{rec}}$, $P$, and $P^{\mathrm{rec}}$. The last term, $B\left(E_\nu^{\mathrm{rec}}, K^{\mathrm{rec}}, P^{\mathrm{rec}}\right)$ represents the estimation of backgrounds as a function of $E_\nu^{\mathrm{rec}}$, $K^{\mathrm{rec}}$, $P^{\mathrm{rec}}$, and also depends on $N$, $T$, $F$, $\sigma$, and the selection strategy.

We can rewrite Eq. (13) in a matrix format:

$$M_{ijk} = \sum_{lmn} \widetilde{S}_{ijklmn} + B_{ijk}, \tag{14}$$

where $i, j, k$ are bin indices in $E_\nu^{\mathrm{rec}}, K^{\mathrm{rec}}$, and $P^{\mathrm{rec}}$, respectively. Similarly, $l, m, n$ are bin indices in true spaces of $E_\nu, K$, and $P$. $\widetilde{S}_{ijklmn}$ is the truth signal corresponding to bin $lmn$ and reconstructed in bin $ijk$.

$$\begin{aligned}
\widetilde{S}_{ijklmn} &= \frac{N \cdot T \cdot \int_{lmn} F\left(E_{\nu\ l}\right) \cdot \frac{d^2\sigma\left(E_{\nu\ l}, K_m, P_n\right)}{dK_m dP_n} \cdot D \cdot \epsilon \cdot dE_{\nu\ l} \cdot dK_m \cdot dP_n}{N \cdot T \cdot \int_{lmn} \overline{F}\left(E_{\nu\ l}\right) \cdot \frac{d^2\sigma\left(E_{\nu\ l}, K_m, P_n\right)}{dK_m dP_n} \cdot dE_{\nu\ l} \cdot dK_m \cdot dP_n} \\
&\cdot \left(N \cdot T \cdot \int_{lmn} \overline{F}\left(E_{\nu\ l}\right) \cdot dE_{\nu\ l} \cdot dK_m \cdot dP_n\right) \\
&\cdot \frac{\int_{lmn} \overline{F}\left(E_{\nu\ l}\right) \cdot \frac{d^2\sigma\left(E_{\nu\ l}, K_m, P_n\right)}{dK_m dP_n} \cdot dE_{\nu\ l} \cdot dK_m \cdot dP_n}{\int_{lmn} \overline{F}\left(E_{\nu\ l}\right) \cdot dE_{\nu\ l} \cdot dK_m \cdot dP_n} \\
&= \Delta_{ijklmn} \cdot F_{lmn} \cdot S_{lmn},
\end{aligned} \tag{15}$$

with

$$\Delta_{ijklmn} \equiv \frac{N \cdot T \cdot \int_{lmn} F\left(E_{\nu\ l}\right) \cdot \frac{d^2\sigma\left(E_{\nu\ l}, K_m, P_n\right)}{dK_m dP_n} \cdot D \cdot \epsilon \cdot dE_{\nu\ l} \cdot dK_m \cdot dP_n}{N \cdot T \cdot \int_{lmn} \overline{F}\left(E_\nu\right) \cdot \frac{d^2\sigma\left(E_{\nu\ l}, K_m, P_n\right)}{dK_m dP_n} \cdot dE_\nu \cdot dK_m \cdot dP_n} \tag{16}$$

being the smearing matrix that can be directly extracted from the simulation:

$$\Delta_{ijklmn} = \frac{\text{Selected no. of events in reco. bin } (i,j,k) \text{ from true bin } (l,m,n) \text{ after event weights}}{\text{Generated no. of events in true bin } (l,m,n) \text{ after event weights}}, \tag{17}$$

which is also used to estimate the impact of various systematic uncertainties (e.g. neutrino flux, neutrino-argon interaction cross section, and detector systematics). Here $\overline{F}$ represents the nominal (or central value) estimation of the $\nu_\mu$ neutrino flux. Furthermore,

$$\begin{aligned}
F_{lmn} &\equiv N \cdot T \cdot \int_{lmn} \overline{F}\left(E_{\nu\ l}\right) \cdot dE_{\nu\ l} \cdot dK_m \cdot dP_n \\
&= N \cdot T \cdot \left(\int_l \overline{F}\left(E_{\nu\ l}\right) \cdot dE_{\nu\ l}\right) \cdot \Delta K_m \cdot \Delta P_n
\end{aligned} \tag{18}$$

is a constant that can be calculated externally knowing the nominal $\nu_\mu$ neutrino flux, the $m$-th bin width $\Delta K_m$ and the $n$-th bin width $\Delta P_n$. Finally, the targeted signal to be unfolded is defined as:

$$S_j \equiv \frac{\int_{lmn} \overline{F}\left(E_{\nu\ l}\right) \cdot \frac{d^2\sigma(E_{\nu\ l}, K_m, P_n)}{dK_m dP_n} \cdot dE_{\nu\ l} \cdot dK_m \cdot dP_n}{\int_{lmn} \overline{F}\left(E_{\nu\ l}\right) \cdot dE_{\nu\ l} \cdot dK_m \cdot dP_n} = \left\langle \frac{d^2\sigma\left(E_{\nu,l}, K_m, P_n\right)}{dK_m dP_n} \right\rangle, \tag{19}$$

and is the flux-averaged three-dimensional cross section of true neutrino energy bin $l$, true $K$ bin $m$ and true $P$ bin $n$ that we pursue in the unfolding procedure. Mapping $R_{ijklmn} = \Delta_{ijklmn} \cdot F_{lmn}$ to Eq. (14), we have

$$M_{ijk} - B_{ijk} = \sum_{lmn} R_{ijklmn} \cdot S_{lmn}. \tag{20}$$

One can concatenate the three indices, and remap $ijk$ and $lmn$ to $i$ and $j$, respectively. As a result, we have

$$M_i - B_i = \sum_j R_{ij} \cdot S_j, \tag{21}$$

which is essentially the master equation in Eq. (12).

## V. CROSS SECTION RESULT DATA RELEASE

The data are compared against each model prediction within individual $E_\nu$ slices, with $\chi^2$ values shown in Table II and Table III. The extracted $\nu_\mu$ CC differential inclusive scattering cross section per argon nucleus as a function of neutrino energy, $d^2\sigma(E_\nu)/d\cos(\theta_\mu)dP_\mu$, is provided in the included root file `microboone_cc_inclusive_cross_section.root` and text file `microboone_cc_inclusive_cross_section.txt`, and in Table IV. The bin ranges over $E_\nu$, $\cos(\theta_\mu)$, and $P_\mu$ are also included. The nominal BNB flux is available in the supplemental material of Ref. [10]. The covariance matrix and additional smearing matrix are provided in the included text files `microboone_cc_inclusive_cov_matrix.txt` and `microboone_cc_inclusive_additional_smearing_matrix.txt`, respectively. The covariance matrix is also shown in Fig. 9, consisting of both statistical and systematic uncertainties and given in units of $(10^{-36}\ \mathrm{cm}^2/\mathrm{GeV/Ar})^2$. The additional smearing is a result of the regularization in the data unfolding procedure, and should be applied to model predictions when comparing to these cross-section results. Figure 10 shows the three-dimensional cross section measurement plotted against the `MicroBooNE model` prediction. Figure 11 shows the data over the two-dimensional distribution of $\{E_\nu, \cos(\theta_\mu)\}$, plotted against the `NuWro` model prediction, with a breakdown of the predicted contributions from different interaction channels. This distribution is constructed from the three-dimensional measurement by integrating over $P_\mu$ and normalizing by the average neutrino energy $\langle E_\nu \rangle$.

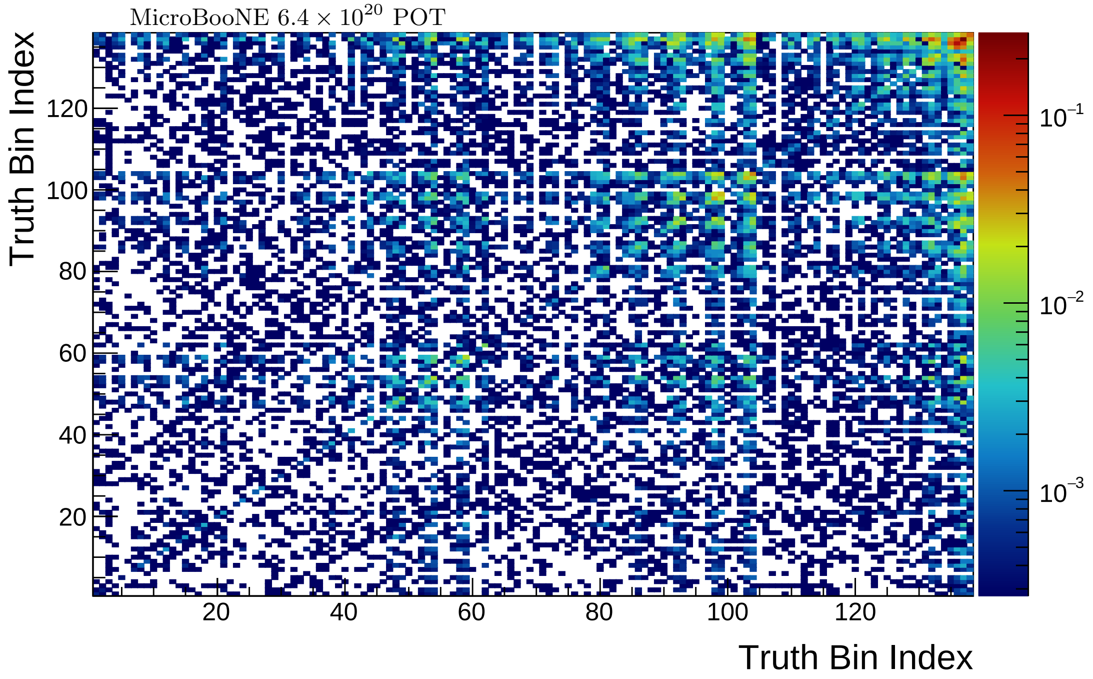


FIG. 9. Covariance matrix showing total statistical plus systematic uncertainties over the 138 measurement bins, in units of $(10^{-36}\ \mathrm{cm}^2/\mathrm{GeV/Ar})^2$. Bins with extremely low values are colored white.

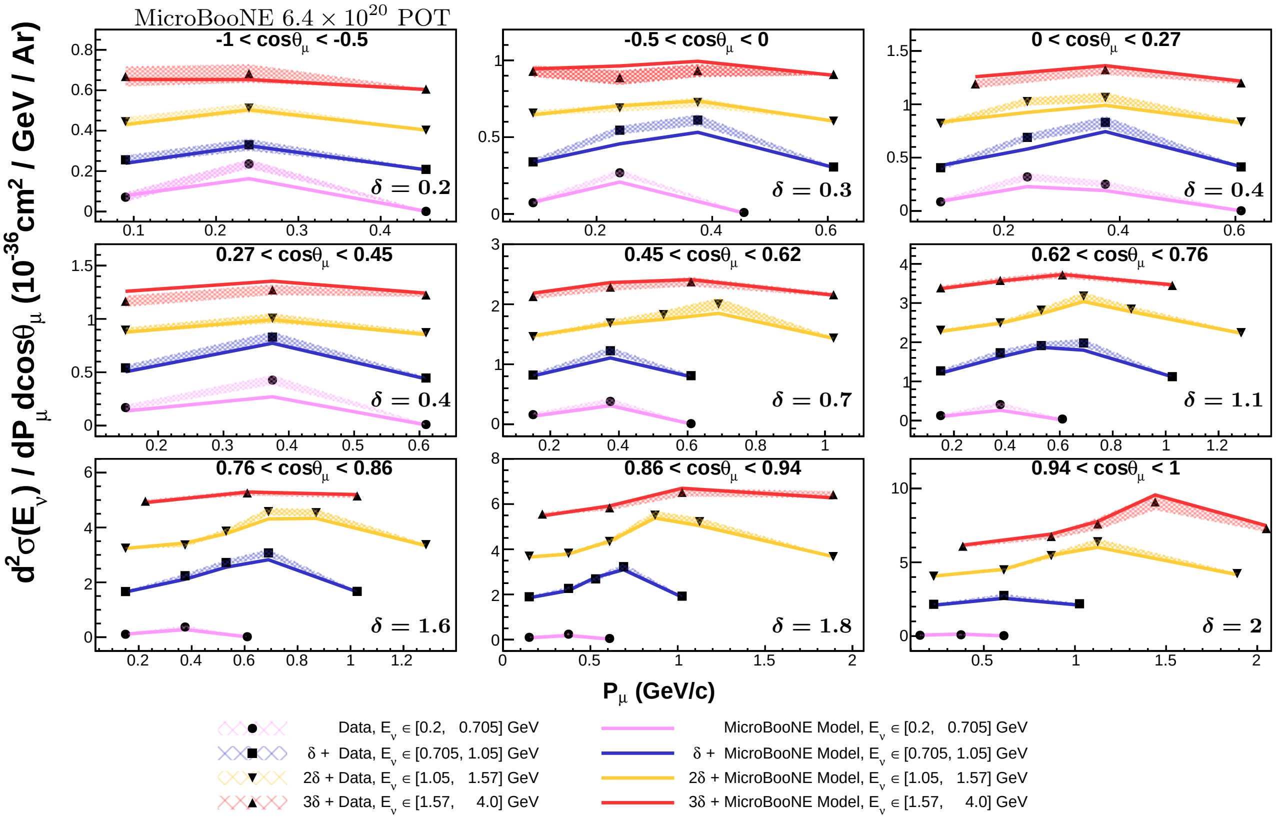


FIG. 10. Unfolded measurement of the inclusive $\nu_\mu$CC differential cross section on argon and `MicroBooNE model` prediction are shown within each angle slice and with each $E_\nu$ measurement overlaid and offset to visually separate them. The magnitude of the offset $\delta$, given in the same units as the cross section, $10^{-36}\mathrm{cm}^2/\mathrm{GeV/Ar}$, is shown in the bottom right of each plot. Uncertainties on the extracted cross section are shown through the shaded bands.

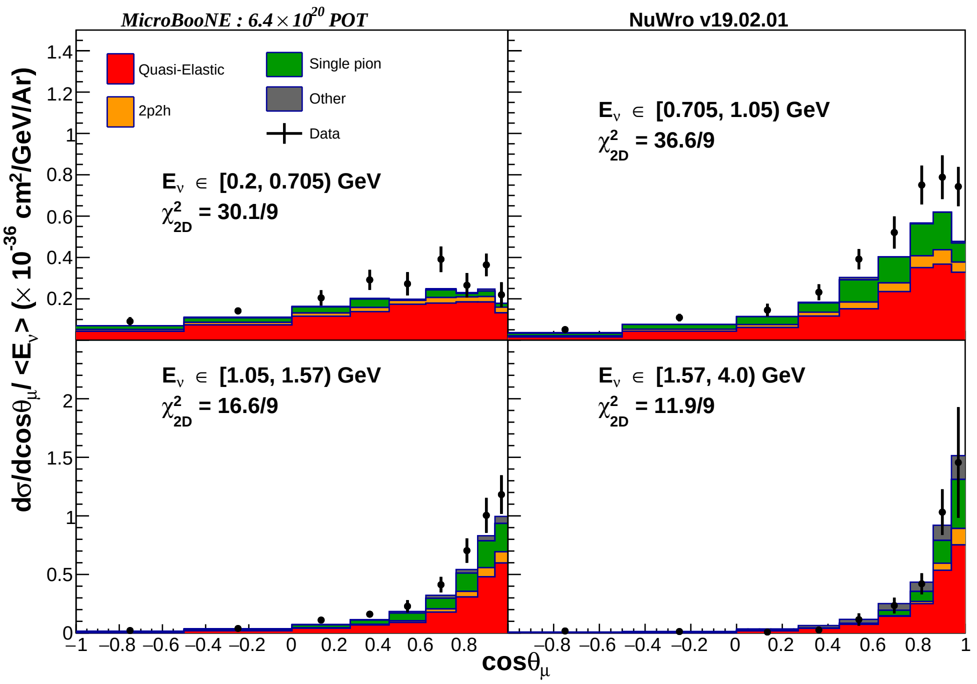


FIG. 11. Unfolded differential cross section over a function of $\cos(\theta_\mu)$ after integrating over $P_\mu$ and normalizing by the average $\langle E_\nu \rangle$ in each $E_\nu$ bin. The NuWro prediction, including a breakdown of interaction channel, is given for comparison.

TABLE II. Comparisons between various models and the unfolded three-dimensional measurement within each $E_\nu$ slice.

| Model Name | Total $\chi^2$/ndf | $[0.2, 0.705]$ GeV $\chi^2$/ndf | $[0.705, 1.05]$ GeV $\chi^2$/ndf | $[1.05, 1.57]$ GeV $\chi^2$/ndf | $[1.57, 4.0]$ GeV $\chi^2$/ndf |
|---|---|---|---|---|---|
| GENIE v2 | 752.2/138 | 69.3/28 | 61.3/35 | 63.0/42 | 34.9/33 |
| MicroBooNE model | 329.3/138 | 88.0/28 | 77.7/35 | 43.5/42 | 31.1/33 |
| GENIE v3 untuned | 324.6/138 | 101.2/28 | 85.2/35 | 50.2/42 | 36.4/33 |
| GiBUU | 275.2/138 | 36.0/28 | 48.7/35 | 53.8/42 | 29.6/33 |
| NEUT | 244.3/138 | 65.3/28 | 58.7/35 | 40.8/42 | 37.0/33 |
| NuWro | 214.1/138 | 60.8/28 | 65.8/35 | 40.3/42 | 28.8/33 |

TABLE III. Comparisons between various models and the unfolded three-dimensional measurement within each $E_\nu$ slice after integrating over the $P_\mu$ dimension.

| Model Name | Total $\chi^2$/ndf | $[0.2, 0.705]$ GeV $\chi^2$/ndf | $[0.705, 1.05]$ GeV $\chi^2$/ndf | $[1.05, 1.57]$ GeV $\chi^2$/ndf | $[1.57, 4.0]$ GeV $\chi^2$/ndf |
|---|---|---|---|---|---|
| GENIE v2 | 125.5/36 | 12.5/9 | 16.6/9 | 20.7/9 | 12.7/9 |
| MicroBooNE model | 87.0/36 | 36.5/9 | 34.8/9 | 12.3/9 | 12.2/9 |
| GENIE v3 untuned | 99.9/36 | 57.3/9 | 55.0/9 | 28.1/9 | 14.0/9 |
| GiBUU | 95.5/36 | 11.4/9 | 13.0/9 | 14.6/9 | 10.3/9 |
| NEUT | 70.5/36 | 32.5/9 | 28.4/9 | 6.8/9 | 16.4/9 |
| NuWro | 75.6/36 | 30.1/9 | 36.6/9 | 16.6/9 | 11.9/9 |

TABLE IV: $\nu_\mu$ CC inclusive differential cross section per argon atom in each neutrino energy bin with total statistical plus systematic uncertainty. The total uncertainty comes from the square root of the covariance matrix diagonal entries.

| Bin Number | $E_\nu$ Range [GeV] | $\cos(\theta_\mu)$ Range | $P_\mu$ Range [GeV] | $\sigma_{\mathrm{MC}}$ $[10^{-36}$ cm$^2$/GeV/Ar$]$ | $\sigma_{\mathrm{Data}}$ $[10^{-36}$ cm$^2$/GeV/Ar$]$ | Total Uncertainty $[10^{-36}$ cm$^2$/Ar$]$ |
|---|---|---|---|---|---|---|
| 0 | [0.2, 0.705] | [-1, -0.5] | [0, 0.18] | 0.079 | 0.071 | 0.023 |
| 1 | [0.2, 0.7] | [-1, -0.5] | [0.18, 0.3] | 0.16 | 0.24 | 0.022 |
| 2 | [0.2, 0.7] | [-1, -0.5] | [0.3, 2.5] | 0.0012 | 0.00064 | 0.0012 |
| 3 | [0.2, 0.7] | [-0.5, 0] | [0, 0.18] | 0.077 | 0.073 | 0.017 |
| 4 | [0.2, 0.7] | [-0.5, 0] | [0.18, 0.3] | 0.21 | 0.27 | 0.020 |
| 5 | [0.2, 0.7] | [-0.5, 0] | [0.3, 2.5] | 0.0066 | 0.0094 | 0.0010 |
| 6 | [0.2, 0.7] | [0, 0.27] | [0, 0.18] | 0.091 | 0.086 | 0.022 |
| 7 | [0.2, 0.7] | [0, 0.27] | [0.18, 0.3] | 0.23 | 0.32 | 0.035 |
| 8 | [0.2, 0.7] | [0, 0.27] | [0.3, 0.45] | 0.19 | 0.25 | 0.031 |
| 9 | [0.2, 0.7] | [0, 0.27] | [0.45, 2.5] | 0.0015 | 0.0019 | 0.0022 |
| 10 | [0.2, 0.7] | [0.27, 0.45] | [0, 0.3] | 0.14 | 0.17 | 0.026 |
| 11 | [0.2, 0.7] | [0.27, 0.45] | [0.3, 0.45] | 0.27 | 0.43 | 0.046 |
| 12 | [0.2, 0.7] | [0.27, 0.45] | [0.45, 2.5] | 0.0069 | 0.010 | 0.0039 |
| 13 | [0.2, 0.7] | [0.45, 0.62] | [0, 0.3] | 0.14 | 0.16 | 0.029 |
| 14 | [0.2, 0.7] | [0.45, 0.62] | [0.3, 0.45] | 0.31 | 0.38 | 0.050 |
| 15 | [0.2, 0.7] | [0.45, 0.62] | [0.45, 2.5] | 0.0050 | 0.011 | 0.0049 |
| 16 | [0.2, 0.7] | [0.62, 0.76] | [0, 0.3] | 0.10 | 0.13 | 0.031 |
| 17 | [0.2, 0.7] | [0.62, 0.76] | [0.3, 0.45] | 0.26 | 0.41 | 0.055 |
| 18 | [0.2, 0.7] | [0.62, 0.76] | [0.45, 2.5] | 0.019 | 0.040 | 0.0055 |
| 19 | [0.2, 0.7] | [0.76, 0.86] | [0, 0.3] | 0.11 | 0.11 | 0.031 |
| 20 | [0.2, 0.7] | [0.76, 0.86] | [0.3, 0.45] | 0.28 | 0.37 | 0.052 |
| 21 | [0.2, 0.7] | [0.76, 0.86] | [0.45, 2.5] | 0.012 | 0.017 | 0.0051 |
| 22 | [0.2, 0.7] | [0.86, 0.94] | [0, 0.3] | 0.081 | 0.10 | 0.024 |
| 23 | [0.2, 0.7] | [0.86, 0.94] | [0.3, 0.45] | 0.18 | 0.24 | 0.041 |
| 24 | [0.2, 0.7] | [0.86, 0.94] | [0.45, 2.5] | 0.024 | 0.050 | 0.0060 |
| 25 | [0.2, 0.7] | [0.94, 1] | [0, 0.3] | 0.069 | 0.060 | 0.034 |
| 26 | [0.2, 0.7] | [0.94, 1] | [0.3, 0.45] | 0.14 | 0.092 | 0.045 |
| 27 | [0.2, 0.7] | [0.94, 1] | [0.45, 2.5] | 0.018 | 0.034 | 0.0055 |
| 28 | [0.7, 1.1] | [-1, -0.5] | [0, 0.18] | 0.039 | 0.056 | 0.021 |
| 29 | [0.7, 1.1] | [-1, -0.5] | [0.18, 0.3] | 0.13 | 0.13 | 0.029 |
| 30 | [0.7, 1.1] | [-1, -0.5] | [0.3, 2.5] | 0.0064 | 0.0085 | 0.0026 |
| 31 | [0.7, 1.1] | [-0.5, 0] | [0, 0.18] | 0.035 | 0.039 | 0.018 |

| | | | | | | |
|---|---|---|---|---|---|---|
| 32 | [0.7, 1.1] | [-0.5, 0] | [0.18, 0.3] | 0.16 | 0.25 | 0.027 |
| 33 | [0.7, 1.1] | [-0.5, 0] | [0.3, 0.45] | 0.23 | 0.31 | 0.036 |
| 34 | [0.7, 1.1] | [-0.5, 0] | [0.45, 2.5] | 0.0031 | 0.0058 | 0.0018 |
| 35 | [0.7, 1.1] | [0, 0.27] | [0, 0.18] | 0.026 | 0.0053 | 0.021 |
| 36 | [0.7, 1.1] | [0, 0.27] | [0.18, 0.3] | 0.18 | 0.29 | 0.035 |
| 37 | [0.7, 1.1] | [0, 0.27] | [0.3, 0.45] | 0.34 | 0.43 | 0.055 |
| 38 | [0.7, 1.1] | [0, 0.27] | [0.45, 2.5] | 0.015 | 0.013 | 0.0050 |
| 39 | [0.7, 1.1] | [0.27, 0.45] | [0, 0.3] | 0.10 | 0.14 | 0.026 |
| 40 | [0.7, 1.1] | [0.27, 0.45] | [0.3, 0.45] | 0.37 | 0.43 | 0.050 |
| 41 | [0.7, 1.1] | [0.27, 0.45] | [0.45, 2.5] | 0.038 | 0.046 | 0.0089 |
| 42 | [0.7, 1.1] | [0.45, 0.62] | [0, 0.3] | 0.11 | 0.12 | 0.030 |
| 43 | [0.7, 1.1] | [0.45, 0.62] | [0.3, 0.45] | 0.41 | 0.53 | 0.060 |
| 44 | [0.7, 1.1] | [0.45, 0.62] | [0.45, 2.5] | 0.092 | 0.11 | 0.012 |
| 45 | [0.7, 1.1] | [0.62, 0.76] | [0, 0.3] | 0.11 | 0.17 | 0.032 |
| 46 | [0.7, 1.1] | [0.62, 0.76] | [0.3, 0.45] | 0.52 | 0.63 | 0.072 |
| 47 | [0.7, 1.1] | [0.62, 0.76] | [0.45, 0.61] | 0.77 | 0.81 | 0.096 |
| 48 | [0.7, 1.1] | [0.62, 0.76] | [0.61, 0.77] | 0.70 | 0.88 | 0.10 |
| 49 | [0.7, 1.1] | [0.62, 0.76] | [0.77, 2.5] | 0.018 | 0.021 | 0.0082 |
| 50 | [0.7, 1.1] | [0.76, 0.86] | [0, 0.3] | 0.047 | 0.065 | 0.022 |
| 51 | [0.7, 1.1] | [0.76, 0.86] | [0.3, 0.45] | 0.51 | 0.64 | 0.073 |
| 52 | [0.7, 1.1] | [0.76, 0.86] | [0.45, 0.61] | 0.95 | 1.1 | 0.095 |
| 53 | [0.7, 1.1] | [0.76, 0.86] | [0.61, 0.77] | 1.2 | 1.5 | 0.13 |
| 54 | [0.7, 1.1] | [0.76, 0.86] | [0.77, 2.5] | 0.054 | 0.070 | 0.015 |
| 55 | [0.7, 1.1] | [0.86, 0.94] | [0, 0.3] | 0.053 | 0.097 | 0.025 |
| 56 | [0.7, 1.1] | [0.86, 0.94] | [0.3, 0.45] | 0.37 | 0.47 | 0.060 |
| 57 | [0.7, 1.1] | [0.86, 0.94] | [0.45, 0.61] | 0.96 | 0.89 | 0.10 |
| 58 | [0.7, 1.1] | [0.86, 0.94] | [0.61, 0.77] | 1.3 | 1.4 | 0.13 |
| 59 | [0.7, 1.1] | [0.86, 0.94] | [0.77, 2.5] | 0.082 | 0.12 | 0.020 |
| 60 | [0.7, 1.1] | [0.94, 1] | [0, 0.45] | 0.095 | 0.16 | 0.035 |
| 61 | [0.7, 1.1] | [0.94, 1] | [0.45, 0.77] | 0.56 | 0.76 | 0.10 |
| 62 | [0.7, 1.1] | [0.94, 1] | [0.77, 2.5] | 0.10 | 0.19 | 0.020 |
| 63 | [1.1, 1.6] | [-1, -0.5] | [0, 0.18] | 0.030 | 0.044 | 0.023 |
| 64 | [1.1, 1.6] | [-1, -0.5] | [0.18, 0.3] | 0.10 | 0.11 | 0.023 |
| 65 | [1.1, 1.6] | [-1, -0.5] | [0.3, 2.5] | 0.0031 | 0.0025 | 0.0019 |
| 66 | [1.1, 1.6] | [-0.5, 0] | [0, 0.18] | 0.046 | 0.057 | 0.017 |
| 67 | [1.1, 1.6] | [-0.5, 0] | [0.18, 0.3] | 0.10 | 0.090 | 0.025 |
| 68 | [1.1, 1.6] | [-0.5, 0] | [0.3, 0.45] | 0.14 | 0.13 | 0.032 |
| 69 | [1.1, 1.6] | [-0.5, 0] | [0.45, 2.5] | 0.0047 | 0.0043 | 0.0023 |
| 70 | [1.1, 1.6] | [0, 0.27] | [0, 0.18] | 0.033 | 0.021 | 0.021 |
| 71 | [1.1, 1.6] | [0, 0.27] | [0.18, 0.3] | 0.12 | 0.22 | 0.036 |
| 72 | [1.1, 1.6] | [0, 0.27] | [0.3, 0.45] | 0.19 | 0.26 | 0.046 |
| 73 | [1.1, 1.6] | [0, 0.27] | [0.45, 2.5] | 0.025 | 0.034 | 0.0060 |
| 74 | [1.1, 1.6] | [0.27, 0.45] | [0, 0.3] | 0.075 | 0.094 | 0.024 |
| 75 | [1.1, 1.6] | [0.27, 0.45] | [0.3, 0.45] | 0.19 | 0.21 | 0.045 |
| 76 | [1.1, 1.6] | [0.27, 0.45] | [0.45, 2.5] | 0.053 | 0.070 | 0.0099 |
| 77 | [1.1, 1.6] | [0.45, 0.62] | [0, 0.3] | 0.076 | 0.060 | 0.027 |
| 78 | [1.1, 1.6] | [0.45, 0.62] | [0.3, 0.45] | 0.27 | 0.29 | 0.048 |
| 79 | [1.1, 1.6] | [0.45, 0.62] | [0.45, 0.61] | 0.35 | 0.43 | 0.064 |
| 80 | [1.1, 1.6] | [0.45, 0.62] | [0.61, 0.77] | 0.45 | 0.60 | 0.097 |
| 81 | [1.1, 1.6] | [0.45, 0.62] | [0.77, 2.5] | 0.032 | 0.036 | 0.013 |
| 82 | [1.1, 1.6] | [0.62, 0.76] | [0, 0.3] | 0.076 | 0.10 | 0.025 |
| 83 | [1.1, 1.6] | [0.62, 0.76] | [0.3, 0.45] | 0.28 | 0.29 | 0.045 |
| 84 | [1.1, 1.6] | [0.62, 0.76] | [0.45, 0.61] | 0.53 | 0.62 | 0.060 |
| 85 | [1.1, 1.6] | [0.62, 0.76] | [0.61, 0.77] | 0.84 | 0.98 | 0.096 |
| 86 | [1.1, 1.6] | [0.62, 0.76] | [0.77, 0.97] | 0.58 | 0.64 | 0.072 |
| 87 | [1.1, 1.6] | [0.62, 0.76] | [0.97, 2.5] | 0.030 | 0.042 | 0.016 |
| 88 | [1.1, 1.6] | [0.76, 0.86] | [0, 0.3] | 0.037 | 0.044 | 0.030 |
| 89 | [1.1, 1.6] | [0.76, 0.86] | [0.3, 0.45] | 0.23 | 0.16 | 0.067 |
| 90 | [1.1, 1.6] | [0.76, 0.86] | [0.45, 0.61] | 0.57 | 0.66 | 0.083 |
| 91 | [1.1, 1.6] | [0.76, 0.86] | [0.61, 0.77] | 1.1 | 1.4 | 0.13 |
| 92 | [1.1, 1.6] | [0.76, 0.86] | [0.77, 0.97] | 1.1 | 1.3 | 0.13 |
| 93 | [1.1, 1.6] | [0.76, 0.86] | [0.97, 2.5] | 0.14 | 0.17 | 0.031 |
| 94 | [1.1, 1.6] | [0.86, 0.94] | [0, 0.3] | 0.056 | 0.092 | 0.024 |
| 95 | [1.1, 1.6] | [0.86, 0.94] | [0.3, 0.45] | 0.19 | 0.22 | 0.048 |

| | | | | | | |
|---|---|---|---|---|---|---|
| 96 | [1.1, 1.6] | [0.86, 0.94] | [0.45, 0.77] | 0.75 | 0.74 | 0.10 |
| 97 | [1.1, 1.6] | [0.86, 0.94] | [0.77, 0.97] | 1.8 | 1.9 | 0.18 |
| 98 | [1.1, 1.6] | [0.86, 0.94] | [0.97, 1.3] | 1.4 | 1.6 | 0.17 |
| 99 | [1.1, 1.6] | [0.86, 0.94] | [1.3, 2.5] | 0.075 | 0.074 | 0.022 |
| 100 | [1.1, 1.6] | [0.94, 1] | [0, 0.45] | 0.068 | 0.058 | 0.039 |
| 101 | [1.1, 1.6] | [0.94, 1] | [0.45, 0.77] | 0.53 | 0.48 | 0.082 |
| 102 | [1.1, 1.6] | [0.94, 1] | [0.77, 0.97] | 1.5 | 1.5 | 0.17 |
| 103 | [1.1, 1.6] | [0.94, 1] | [0.97, 1.3] | 2.0 | 2.4 | 0.20 |
| 104 | [1.1, 1.6] | [0.94, 1] | [1.3, 2.5] | 0.17 | 0.23 | 0.034 |
| 105 | [1.6, 4] | [-1, -0.5] | [0, 0.18] | 0.053 | 0.068 | 0.049 |
| 106 | [1.6, 4] | [-1, -0.5] | [0.18, 0.3] | 0.053 | 0.083 | 0.045 |
| 107 | [1.6, 4] | [-1, -0.5] | [0.3, 2.5] | 0.0035 | 0.0055 | 0.0019 |
| 108 | [1.6, 4] | [-0.5, 0] | [0, 0.18] | 0.044 | 0.029 | 0.036 |
| 109 | [1.6, 4] | [-0.5, 0] | [0.18, 0.3] | 0.063 | -0.012 | 0.046 |
| 110 | [1.6, 4] | [-0.5, 0] | [0.3, 0.45] | 0.094 | 0.033 | 0.041 |
| 111 | [1.6, 4] | [-0.5, 0] | [0.45, 2.5] | 0.0027 | 0.0079 | 0.0043 |
| 112 | [1.6, 4] | [0, 0.27] | [0, 0.3] | 0.058 | -0.0092 | 0.039 |
| 113 | [1.6, 4] | [0, 0.27] | [0.3, 0.45] | 0.16 | 0.12 | 0.048 |
| 114 | [1.6, 4] | [0, 0.27] | [0.45, 2.5] | 0.017 | 0.00036 | 0.011 |
| 115 | [1.6, 4] | [0.27, 0.45] | [0, 0.3] | 0.059 | -0.034 | 0.051 |
| 116 | [1.6, 4] | [0.27, 0.45] | [0.3, 0.45] | 0.15 | 0.072 | 0.049 |
| 117 | [1.6, 4] | [0.27, 0.45] | [0.45, 2.5] | 0.042 | 0.025 | 0.017 |
| 118 | [1.6, 4] | [0.45, 0.62] | [0, 0.3] | 0.085 | 0.029 | 0.042 |
| 119 | [1.6, 4] | [0.45, 0.62] | [0.3, 0.45] | 0.26 | 0.19 | 0.057 |
| 120 | [1.6, 4] | [0.45, 0.62] | [0.45, 0.77] | 0.31 | 0.27 | 0.076 |
| 121 | [1.6, 4] | [0.45, 0.62] | [0.77, 2.5] | 0.052 | 0.058 | 0.032 |
| 122 | [1.6, 4] | [0.62, 0.76] | [0, 0.3] | 0.067 | 0.088 | 0.048 |
| 123 | [1.6, 4] | [0.62, 0.76] | [0.3, 0.45] | 0.26 | 0.28 | 0.071 |
| 124 | [1.6, 4] | [0.62, 0.76] | [0.45, 0.77] | 0.43 | 0.42 | 0.083 |
| 125 | [1.6, 4] | [0.62, 0.76] | [0.77, 2.5] | 0.17 | 0.15 | 0.044 |
| 126 | [1.6, 4] | [0.76, 0.86] | [0, 0.45] | 0.11 | 0.16 | 0.050 |
| 127 | [1.6, 4] | [0.76, 0.86] | [0.45, 0.77] | 0.49 | 0.46 | 0.095 |
| 128 | [1.6, 4] | [0.76, 0.86] | [0.77, 2.5] | 0.40 | 0.35 | 0.069 |
| 129 | [1.6, 4] | [0.86, 0.94] | [0, 0.45] | 0.079 | 0.16 | 0.058 |
| 130 | [1.6, 4] | [0.86, 0.94] | [0.45, 0.77] | 0.52 | 0.44 | 0.11 |
| 131 | [1.6, 4] | [0.86, 0.94] | [0.77, 1.3] | 1.3 | 1.1 | 0.18 |
| 132 | [1.6, 4] | [0.86, 0.94] | [1.3, 2.5] | 0.88 | 1.0 | 0.15 |
| 133 | [1.6, 4] | [0.94, 1] | [0, 0.77] | 0.16 | 0.089 | 0.073 |
| 134 | [1.6, 4] | [0.94, 1] | [0.77, 0.97] | 0.91 | 0.75 | 0.17 |
| 135 | [1.6, 4] | [0.94, 1] | [0.97, 1.3] | 1.8 | 1.6 | 0.40 |
| 136 | [1.6, 4] | [0.94, 1] | [1.3, 1.6] | 3.6 | 3.1 | 0.55 |
| 137 | [1.6, 4] | [0.94, 1] | [1.6, 2.5] | 1.5 | 1.3 | 0.23 |


[1] C. Rasmussen *et al.*, *Gaussian Processes for Machine Learning (Adaptive Computation and Machine Learning)* (The MIT Press, 2005).

[2] M. Frate *et al.*, Modeling Smooth Backgrounds and Generic Localized Signals with Gaussian Processes, (2017), arXiv:1709.05681 [physics.data-an].

[3] L. Li *et al.*, Efficient neutrino oscillation parameter inference using Gaussian processes, Phys. Rev. D **101**, 012001 (2020).

[4] P. Abratenko *et al.* (MicroBooNE Collaboration), Search for an anomalous excess of inclusive charged-current $\nu_e$ interactions in the MicroBooNE experiment using Wire-Cell reconstruction, Phys. Rev. D **105**, 112005 (2022).

[5] P. Abratenko *et al.* (MicroBooNE Collaboration), Novel approach for evaluating detector-related uncertainties in a LArTPC using MicroBooNE data, The Eur. Phys. J. C **82**, 454 (2022).

[6] P. Abratenko *et al.* (MicroBooNE Collaboration), First Simultaneous Measurement of Differential Muon-Neutrino Charged-Current Cross Sections on Argon for Final States with and without Protons Using MicroBooNE Data, Phys. Rev. Lett. **133**, 041801 (2024).

[7] M. Eaton, Multivariate statistics: a vector space approach, John Wiley and Sons , 116 (1983).

[8] P. Abratenko *et al.* (MicroBooNE Collaboration), First Measurement of Energy-Dependent Inclusive Muon Neutrino Charged-Current Cross Sections on Argon with the MicroBooNE Detector, Phys. Rev. Lett. **128**, 151801 (2022).

[9] P. Abratenko *et al.* (MicroBooNE Collaboration), Inclusive cross section measurements in final states with and without protons for charged-current $\nu_\mu$-Ar scattering in MicroBooNE, Phys. Rev. D **110**, 013006 (2024).

[10] P. Abratenko *et al.* (MicroBooNE Collaboration), First Measurement of Inclusive Muon Neutrino Charged Current Differential Cross Sections on Argon at $E_\nu \sim 0.8$ GeV with the MicroBooNE Detector, Phys. Rev. Lett. **123**, 131801 (2019), arXiv:1905.09694.
